# Supplementary material for: Precise Knowledge Transfer via Flow Matching
Source: arXiv:2402.02012 source file (2024-02-03)
Supplement: Supplementary file 1 [file additional_offline_coco_comparsion.tex]

\setlength{\tabcolsep}{4pt}
\begin{table}[!t]
\tiny

\begin{center}
\resizebox{0.8\textwidth}{!}{%
\begin{tabular}{lclccccc}
\shline
Method & Schedule & mAP & AP$_\textrm{50}$ & AP$_\textrm{75}$ & AP$_\textrm{S}$ & AP$_\textrm{M}$ & AP$_\textrm{L}$  \\
\hline
\noalign{\smallskip}
Retina-ResX101 (T) & 2$\times$ & 40.8 & 60.5 & 43.7 & 22.9 & 44.5 & 54.6 \\
Retina-Res50   (S) & 2$\times$ & 37.4 & 56.7 & 39.6 & 20.0 & 40.7 & 49.7 \\
FKD & 2$\times$ & 39.6 (+2.2) & 58.8 & 42.1 & 22.7 & 43.3 & 52.5 \\
FRS & 2$\times$ & 40.1 (+2.7) & 59.5 & 42.5 & 21.9 & 43.7 & 54.3 \\
FGD & 2$\times$ & 40.4 (+3.0) & 59.9 & 43.3 & \textbf{23.4} & 44.7 & 54.1 \\
PKD & 2$\times$ & \textbf{40.8 (+3.4)} & \textbf{60.3} & \textbf{43.4} & 23.0 & \textbf{45.1} & \textbf{54.7} \\
MS-KD ($K$=1) & - & - & - & - & - & - & - \\
MS-KD ($K$=4) & - & - & - & - & - & - & - \\
\shline
\end{tabular}}
\vspace{-10pt}
\end{center}
\caption{Additional results of FM-KT with different detection frameworks on MS-COCO. T and S mean the teacher and student detector, respectively.}
\label{tab:add_ms_coco_results}
\vspace{-20pt}
\end{table}
